# Supplementary material for: Beta Regression with Autoregressive Errors for Interrupted Time Series Analysis of Proportion and Rate Outcomes: A Simulation Study
Source: arXiv:2607.07914 source file (2026-10-26)
Supplement: Supplementary file 1 [file supplement.tex]

\documentclass[11pt]{article}
\usepackage[margin=1in]{geometry}
\usepackage{amsmath,amssymb}
\usepackage{booktabs}
\usepackage{longtable}
\usepackage{caption}
\usepackage[colorlinks=true,citecolor=blue,linkcolor=blue]{hyperref}

\title{Supplementary Material\\[4pt]\large Beta Regression with Autoregressive Errors for Interrupted Time Series Analysis of Proportion and Rate Outcomes: A Simulation Study}
\author{Ariel Linden, DrPH}
\date{}

\begin{document}
\maketitle

\renewcommand{\thetable}{S\arabic{table}}
\setcounter{table}{0}

\section*{Appendix A: Preliminary Dispersion (cv) Sensitivity Evaluation}

Prior to the primary simulation, a preliminary Monte Carlo evaluation examined whether the dispersion of the simulated series, controlled through the target coefficient of variation $\mathrm{cv}$ (equation~7 of the main text), introduces bias into the recovered slope-change coefficient. Because the recursive AR($k$) substitution underlying both the data-generating process and the \texttt{betark} likelihood (equation~3 of the main text) builds the autoregressive feedback term from \emph{realized}, link-transformed lagged outcomes rather than a mean-zero latent error, the expectation of the logit-transformed outcome does not equal the logit of its conditional mean for finite precision $\phi$; this gap is largest when $\mu_t$ is far from $0.5$ and $\phi$ is small (i.e., $\mathrm{cv}$ is large), and propagates through the autoregressive recursion. This preliminary evaluation was conducted under a single representative scenario -- AR(2) mild-positive autocorrelation ($\rho = (0.4, 0.2)$), intercept $\mu_0=.10$, a $20\%$ immediate level change, and a $10\%$ post-intervention trend, $T=300$ -- across four dispersion levels.

Table~\ref{tab:S1} reports the bias in the slope-change coefficient as a proportion of its true value. The $\mathrm{cv}=.10$ and $\mathrm{cv}=.20$ rows are averaged across 100 Monte Carlo replications. The $\mathrm{cv}=.05$ and $\mathrm{cv}=.30$ rows reflect single-replication illustrative runs conducted earlier in model development, prior to the adoption of a fully averaged Monte Carlo protocol, and are reported here for completeness and because they are consistent with the monotonic trend established by the two averaged points; they should be interpreted as illustrative rather than as independently confirmed Monte Carlo evidence. Based on the two averaged points and the consistent monotonic pattern across all four, $\mathrm{cv} \le .10$ was judged adequate to keep bias in the slope-change coefficient below approximately $4\%$ of its true value, motivating the choice of $\mathrm{cv}=.05$ for the primary simulation (main text, Section 2.4.1).

\begin{table}[htbp]
\centering
\caption{Bias in the slope-change coefficient as a function of dispersion (cv), AR(2) mild-positive scenario.}
\label{tab:S1}
\begin{tabular}{lccc}
\toprule
$\mathrm{cv}$ & Implied $\phi$ & Bias (proportion of true value) & Replications \\
\midrule
0.05 & 3{,}599 & 0.027 & 1 (illustrative) \\
0.10 & 899     & 0.038 & 100 \\
0.20 & 224     & 0.103 & 100 \\
0.30 & 99      & 0.215 & 1 (illustrative) \\
\bottomrule
\end{tabular}
\end{table}

\clearpage
\section*{Appendix B: Misspecification Analysis (Full Results)}

Table~\ref{tab:S2} reports the full misspecification results: \texttt{betark} fit with the correct AR order, one lag under-specified, and (where applicable) one lag over-specified, under the mild-positive autocorrelation scenario at each true AR order, with the post-intervention trend effect fixed at $50\%$ (500 replications per cell; the GLM+HAC comparator is not included, since its HAC correction does not require specifying an AR order).

\begingroup
\small
\input{tableS2.tex}
\endgroup

\clearpage
\section*{Appendix C: Sensitivity Analysis (Full Results)}

Table~\ref{tab:S3} reports the full sensitivity results across all four starting means and three pre-intervention trend conditions, with the autoregressive structure held fixed at AR(1) Scenario 1 ($\rho=0.4$) and $T=200$ throughout (500 replications per cell). Following the null/non-null separation applied throughout the main text, Type~I error is reported from the null ($0\%$ post-intervention trend) replications only; bias, the standard error ratio, 95\% coverage, and power are reported from the non-null ($50\%$) replications only.

\begingroup
\small
\input{tableS3.tex}
\endgroup

\end{document}
